# Supplementary material for: Probing magnetism in exfoliated VI$_3$ layers with magnetotransport
Source: arXiv:2204.10010 ancillary file (2022-08-03)
Supplement: Supplementary file 1 [file supp_DSDVI3.pdf]

# Supporting Information: Probing magnetism in exfoliated $VI_3$ layers with magnetotransport

David Soler-Delgado,[1,2] Fengrui Yao,[1,2] Dumitru Dumcenco,[1] Enrico Giannini,[1] Jiaruo Li,[3] Connor A. Occhialini,[3] Riccardo Comin,[3] Nicolas Ubrig,[1,2] and Alberto F. Morpurgo[1,2,*]

[1] *Department of Quantum Matter Physics, University of Geneva, 24 Quai Ernest Ansermet, CH-1211 Geneva, Switzerland*

[2] *Group of Applied Physics, University of Geneva, 24 Quai Ernest Ansermet, CH-1211 Geneva, Switzerland*

[3] *Department of Physics, Massachusetts Institute of Technology, Cambridge, Massachusetts 02139, USA*

(Dated: August 3, 2022)

## CONTENTS

Section S1. Methods 2

Section S2. Reproducibility of the magnetoconductance measurements in different devices 3

Section S3. Bias independent magnetoconductance 8

* alberto.morpurgo@unige.ch

## Section S1. METHODS

*Crystal Growth*

Crystals of $VI_3$ were grown using the Physical Vapour Transport method. Stoichiometric amounts of Iodine lumps (99.999 % ultra-dry, Alfa Aesar) and Vanadium powder (+99.5 %, Chempur) were mixed and put inside a quartz tube of internal diameter 0.8 cm and length 14 cm, that was repeatedly evacuated and flushed with pure Ar, then sealed in vacuum. The tube was placed in a tubular furnace, under a temperature gradient with the hot end at 400° C and the cold end at 330°-350° C, for six days. At the end of the treatment, large, shiny, plate-like crystals were found at the cold end of the tube, and extracted. All the manipulations were done inside a glove box under pure Ar atmosphere. Due to the strong sensitivity of $VI_3$ to moisture, the crystals were mounted in a tight sample holder under inert atmosphere for the structural characterization. X-ray diffraction and Energy Dispersive X-ray spectroscopy confirmed the structural and chemical purity of the samples. The magnetic characterization was carried out in a MPMS3 SQUID magnetometer (Quantum Design). The D.C. magnetic moment of $VI_3$ was measured in both orientation of the applied field, either parallel or perpendicular to the ab crystallographic plane, as a function of the applied field and temperature. Some of the resulting data are shown in Figure 1 of the main text.

*Transport Measurements*

All transport measurements were performed in a Heliox 3He insert system (Oxford Instruments) equipped with a superconducting magnet. The lowest temperature measured was 4K and the highest applied magnetic field was 8 T. To measure the I-V characteristics of both, transistor the tunnel barrier devices and their magnetoresistances, the bias voltage was applied using a home-made low noise source. The current and voltage signals were amplified with home-made low noise electronics and the amplified signals were recorded with an Agilent 34410A digital multimeter unit. When measuring the transistor devices, a Keithley 2400 source/measure was used to apply the gate voltage.

*Reflective Magnetic Circular Dichroism Measurements.*

RMCD measurements were performed using a photoelastic modulator (PEM) and a lock-in amplifier. The output of a Helium-Neon laser ($\lambda$ = 633 nm) is first amplitude modulated using a mechanical chopper. The beam is then sent through the PEM, linearly polarized at 45 degrees with respect to the PEM fast axis. The PEM is set to quarter-wave retardance

amplitude for polarization-modulation between right-/left-circular polarization (RCP/LCP) at the fundamental frequency of the PEM (f = 50 kHz). This light is focused onto the sample using a 50x magnification objective lens with an incident average power on the sample of $\sim 20\ \mu$W and a 2 $\mu$m radius spot size. The reflected light is collected using a non-polarizing beamsplitter and recorded by an amplified photodiode.

The collected signal is sent to two lock-in amplifiers, one referenced to the chopper frequency, and the other to the first harmonic of the PEM modulation frequency. The lock-in amplifiers respectively measure the total intensity of the reflected beam, and the circular dichroism (CD), related to the difference in reflectance between RCP and LCP light. The reported MCD signal is then the ratio of the CD and total intensity signals.

Magnetic field and variable temperature were achieved using a Montana Instruments closed-cycle optical cryostat. Field-cooled magnetization measurements were performed with a starting temperature of 100 K, above the ferromagnetic transition. A field of $\pm$980 mT is applied and the sample is cooled to 20 K. The field is then shut off and the RMCD signal is recorded as a function of increasing temperature.

## Section S2. REPRODUCIBILITY OF THE MAGNETOCONDUCTANCE MEASUREMENTS IN DIFFERENT DEVICES

In the main manuscript we present magnetoconductance measurements performed on a $VI_3$ transistor and on a tunnel-junction device, and we state that the data are representative of the behavior of all devices measured. For completeness, here we show data from an additional transistor device and for three other tunnel junction devices, which substantiate our claim regarding the reproducibility of the experimental results.

The two transistor devices that we have studied were fabricated using $VI_3$ exfoliated layers that are repsectively 20 nm and 4.3 nm thick. In the main text, we extensively discuss in-plane transport measurements performed on the 20 nm device, and in Fig. S2 we show data taken on the 4.3 nm device. In contrast to the device shown in the main text, which

employed a back gated with 285 nm thick $SiO_2$ layer (in addition to the thin hBN layer used for encapsulation, see Fig. 1a in the main text), in the 4.3 nm thick device we employed a top gate separated from $VI_3$ by only the hBN layer (30 nm thick) used for encapsulation. Figure S1a shows the transfer curve ($I_{SD}$-vs-$V_G$) measured at fixed $V_{SD} = 8$ V at $T = 60$ K. Identically to what we have shown in the text for the 20 nm thick device, a positive gate voltage $V_G$ enhances the current, due to the accumulation of electrons at the surface of $VI_3$. The gate voltage range is smaller as compared to the one used to study the 20 nm thick devices (see Fig. 1b in the main text) because the thinner gate insulator results in a larger gate capacitance.

The in-plane magnetoconductance $\delta G = (G(H_\perp, T) - G(0,T))/G(0,T)$ of the 4.3 nm thick devices measured as a function of perpendicular magnetic field and temperature $T$ is shown in Fig. S1b as color plot. Overall, the data are virtually identical to those measured on the 20 nm thick device shown in Fig. 1e of the main text, and exhibit the charac-

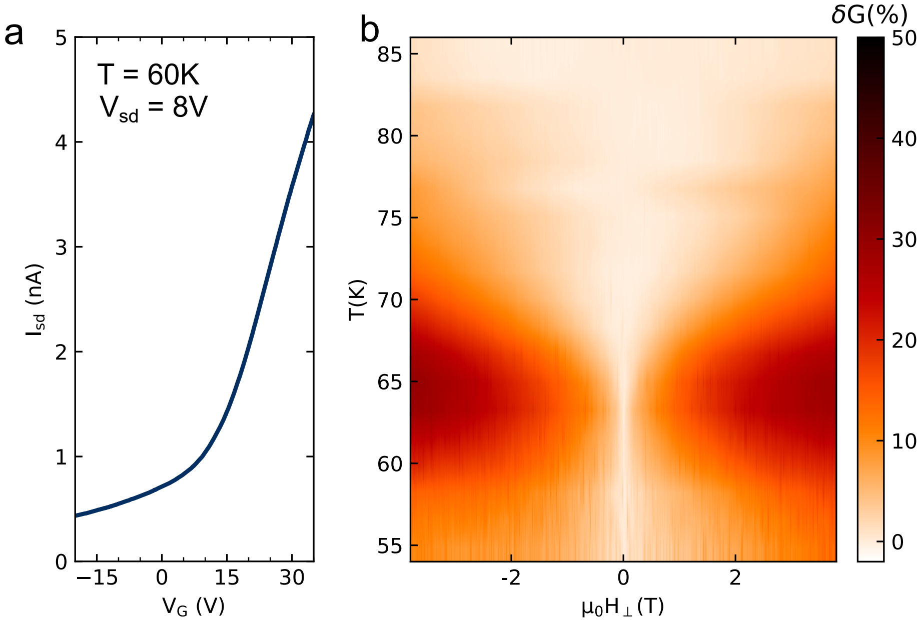


FIG. S1. Transfer curve $I_{sd}$-vs-$V_G$ **(a)**, and color plot of the in-plane magnetoconductance $\delta G$ as a function of the magnetic field $\mu H_\perp$ applied along the c-axis and temperature $T$ **(b)**, for the 4.3 nm transistor device. The transfer curve was measured at fixed $V_{SD} = 8$ V and $T = 60$ K. The color plot, which it is an interpolation of the data measured every 2K, shows the characteristics *lobes* corresponding to the paramagnetic-ferromagnetic transition at $T_C = 60$ K.

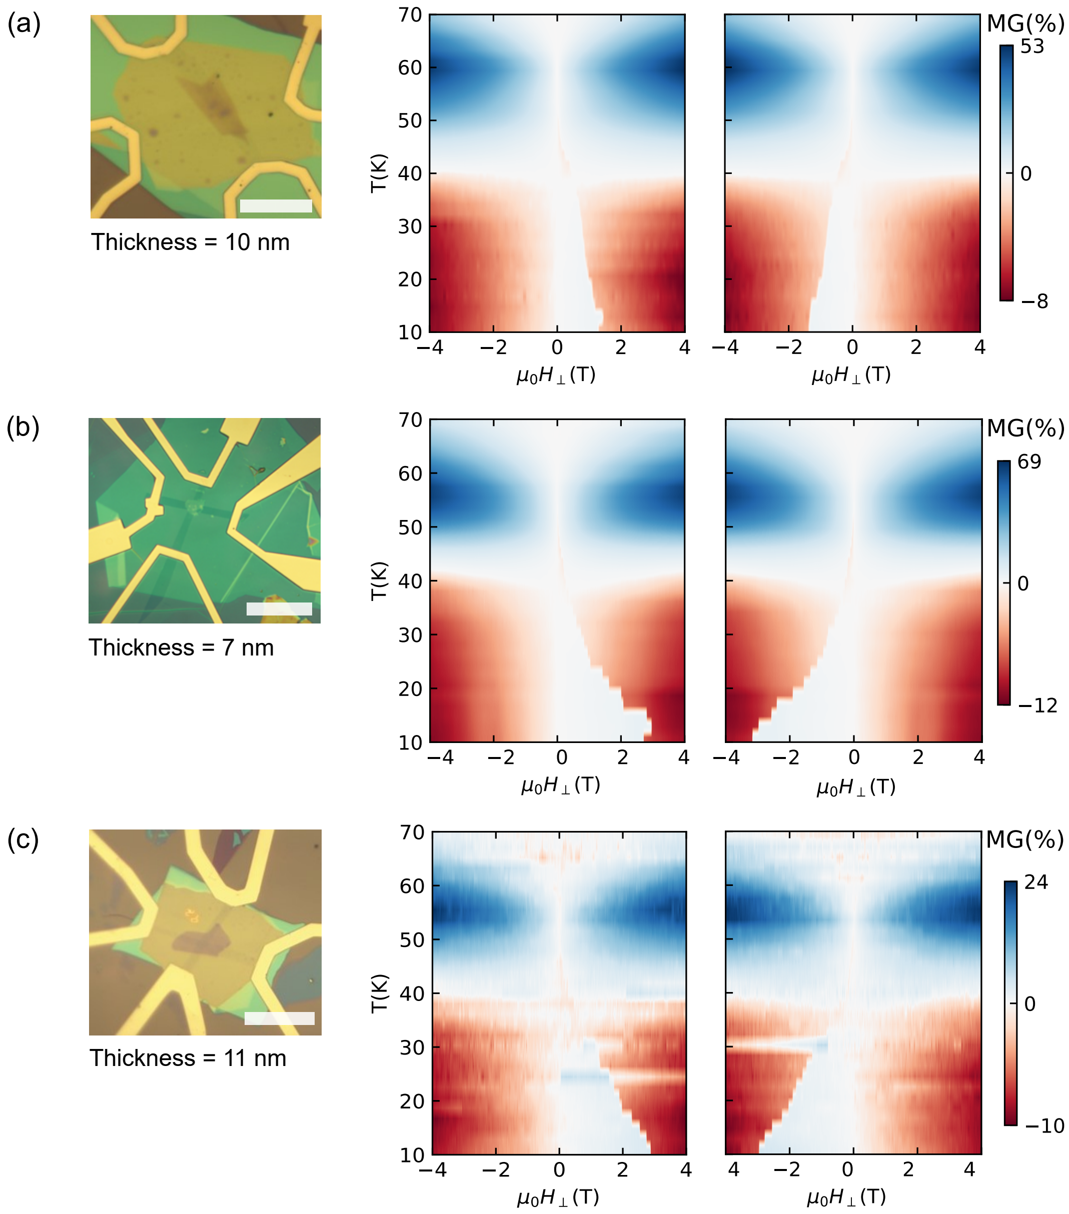


FIG. S2. Optical micrograph and color plot of the tunneling magnetoconductance $\delta G$ as a function of the applied field perpendicularly to the ab-plane $\mu_0 H_\perp$ and temperature $T$ for a 10 nm device **(a)**, a 7 nm device **(b)** and a 11 nm device **(c)**. Left and Right panels represent the magnetoconductance measured by sweeping the field in the positive and negative directions, respectively. Despite the device based on the 11 nm thick layers appears to be less stable than the other devices (At several magnetic fields the magnetoconductance is seen to unexpectedly switch due to a possible contact problem), it exhibits all the characteristic features of tunneling in a perpendicular field that we discuss in the main text and that are reproducible in the other devices. The white scale bar in the optical micro-graphs represents 10 $\mu$m.

teristic "lobes" of enhanced magnetoconductance, associated to the critical regime near the paramagnetic-to-ferromagnetic transition. By scaling the magnetoconductance as a function of the magnetization $M = \mu_0 H/(T - T_\mathrm{C})$ we determine the transition temperature in this device to be $T_\mathrm{C} = 60$ K, 3 K higher than the device presented in the main text. The reason for this small discrepancy is unclear, as in all other devices –transistor or tunnel junctions– we found $T_\mathrm{C} = 57$ K. Despite this small discrepancy, our measurements in both transistor devices show consistently the occurrence of a transition of paramagnetic to ferromagnetic phases in exfoliated $VI_3$ and demonstrate the possibility to use the in-plane transport measurements to probe magnetism in atomically thin materials.

As for the tunneling devices, we measured a total of four tunnel junctions, based on $VI_3$ crystals with thickness ranging from 7 nm to 18 nm. The discussion in the main text is based on data measured on one of these devices, and here we show selected data from the other three devices. Figure S2 shows optical microscope images and full dependence of the tunneling magnetoconductnace $\delta G(H_\perp, T) = (G(H_\perp, T) - G(0, T))/G(0, T)$ as a function of temperature, $T$, and magnetic field applied perpendicular to the layers, $\mu_0 H_\perp$ for a 10 nm device (panel a), a 7 nm device (panel b) and a 11 nm device (panel c). In each panel, left and right plots represent the magnetoconductance measured while sweeping the field from -4 T to +4 T, or from +4 T to -4 T, respectively. The overall behavior is virtually identical to that seen in the device discussed in the main text (i.e., Figure 3 of the main text). From each set of data, the two temperatures of our interest can be easily identified. One is the ferromagnetic transition temperature at $T_\mathrm{C}$ ( identified by the "lobes" in magnetoconductance), always close to 57 K within the precision of the measurements, determined by the step in temperature with which magnetoconductance measurements are taken. The other is the temperature at which magnetoconductnace changes sign, which varies between 36 K and 40 K in different devices.

Finally, Fig. S3 shows the tunneling magnetoconductance with the applied field parallel with the ab-plane $\delta G(\mu_0 H_\parallel)$ for two of the devices whose data are shown in Fig. S2 (the 10 nm device in panel a and the 7 nm device in panel b. We skip the in-plane measurements for the 11 nm device owing to its poorer stability; see Fig. S2c). In each panel, the left columns shows the full dependence of the tunneling magnetoconductance as a function of

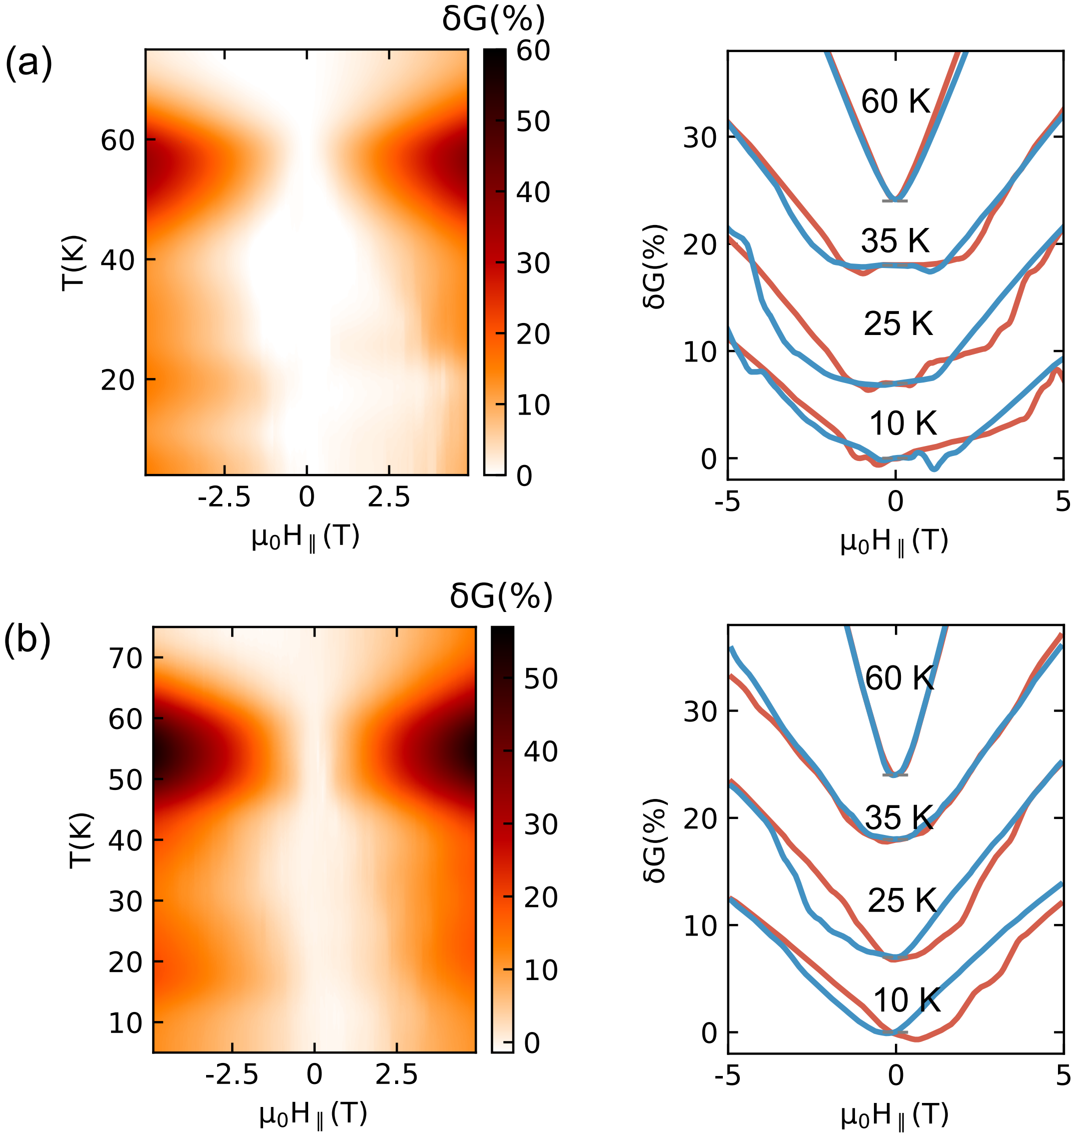


FIG. S3. Color plot of the tunneling magnetoconductance $\delta G$ as a function of the field applied parallel to the ab-plane $\mu_0 H_{\parallel}$ and temperature $T$, and individual traces of $\delta G(\mu_0 H_{\perp})$ at different temperatures (T = 10 K, 25 K, 35 K and 60 K) for a 10 nm device, **(a)** and 7 nm device **(b)**. Red and blue traces in the rightmost panels represent the magnetoconductance measured while sweeping the field in the positive and negative direction, respectively. Owing to the poorer statbility of the tunnel junction based on the 11 nm thick $VI_3$ layer (see Fig.S2c), we have not measured its tunneling magnetoconductance with the in-plane field.

magnetic field $\mu_0 H_{\parallel}$ and temperature $T$, and the right column shows plots of individual $\delta G$

traces at selected temperatures. As it can be checked by a direct comparison with Fig. 5 in the main text, also with the magnetic field applied parallel to the plane, the behavior of these two additional devices is virtually identical to the behavior of the device discussed in the main text.

### Section S3. BIAS INDEPENDENT MAGNETOCONDUCTANCE

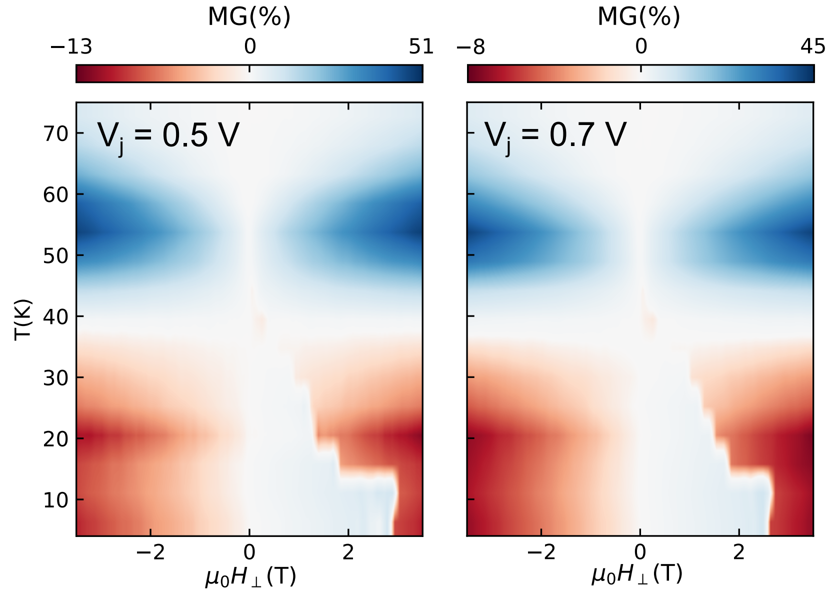


FIG. S4. Color plots of the tunneling magnetoconductance $\delta G$ as a function of temperature $T$ and magnetic field applied perpendicularly to the ab-plane $\mu_0 H_\perp$ measured at two different applied potential across the junction, for the device shown in the main text. The data was taken from 4 to 75 K in a 5 K step. Since the tunneling $I-V$ curves are non-linear, the absolute value of the magnetoconductance depends on the bias conditions. However, all qualitative features discussed in the main text, namely the appearance of ferromagnetic transition and the crossover from positive-negative magneto conductance are bias independent allowing us to draw conclusions on the magnetic state of $VI_3$ through tunneling experiments.

As discussed in the main text, the tunneling mangetoconductance is a powerful technique to probe the magnetic state of exfoliated thin crystals. However, the tunneling $I-V$ curves are extremely non-linear and the absolute value of the measured conductance strongly depends on the applied bias voltage. It is therefore important to check that the magneto-

conductance exhibits the same behavior irrespective of the applied voltage at which measurements are done (i.e., that the absolute value of the conductance has no influence on the conclusions extracted from the data). To this end, in Fig S4a and b, we compare the magnetoconductance of the device presented in the main text plotted as function of the magnetic field and the temperature, as calculated from conductance measurements performed at two different values of applied voltage ($V_j$ = 0.5 V and $V_j$ =0.7 V, respectively). The most important qualitative features, *i.e.*, the sign change of the magnetoconductance with decreasing temperature and the magnetoconductance *lobes* at $T_{\mathrm{C}}$, are completely insensitive to the bias at which the measurements are performed. We therefore conclude that the magnetoconductance measurements can be used to extract information about the magnetic state of $VI_3$ exfoliated multilayers, irrespective of the voltage at which data are taken.
